# Supplementary material for: Data-driven Distributed and Localized Model Predictive Control
Source: arXiv:2112.12229 source file (2021-12-22)
Supplement: Supplementary file 1 [file 9-appendix.tex]

\section*{Appendix}
